# Supplementary material for: Berezinskii-Kosterlitz-Thouless region and magnetization plateaus in easy-axis triangular weak-dimer antiferromagnet K$_2$Co$_2$(SeO$_3$)$_3$
Source: arXiv:2501.09619 source file (2025-01-23)
Supplement: Supplementary file 1 [file KCoSeO_SM.pdf]

# Supplementary Materials for "Berezinskii-Kosterlitz-Thouless region and magnetization plateaus in easy-axis triangular weak-dimer antiferromagnet $K_2Co_2(SeO_3)_3$"

Ying Fu,[1,2] Han Ge,[2] Jian Chen,[2] Jie Xiao,[2] Yi Tan,[2] Le Wang,[3] Junfeng Wang,[4] Chao Dong,[4]
Zhe Qu,[5,6] Miao He,[5,6] Chuanying Xi,[6] Langsheng Ling,[6] Bin Xi,[7,*] and Jia-Wei Mei[2,†]

[1]*Quantum Science Center of Guangdong-Hong Kong-Macao Greater Bay Area (Guangdong), Shenzhen 518045, China*
[2]*Department of Physics, Southern University of Science and Technology, Shenzhen 518055, China*
[3]*International Quantum Academy, Shenzhen, 518048, China*
[4]*Wuhan National High Magnetic Field Center, Huazhong University of Science and Technology, Wuhan 430074, China*
[5]*Science Island Branch of Graduate School, University of Science and Technology of China, Hefei, Anhui, 230026, China*
[6]*Anhui Key Laboratory of Low-Energy Quantum Materials and Devices, High Magnetic Field Laboratory, HFIPS, Chinese Academy of Sciences, Hefei, Anhui 230031, China*
[7]*College of Physics Science and Technology, Yangzhou University, Yangzhou 225002, China*

(Dated: January 23, 2025)

## Contents

I. High-field magnetization measurements 2

II. Specific heat analysis 3

III. Detailed thermodynamic measurements 4

IV. Classical Monte Carlo simulations 6

* xibin@yzu.edu.cn
† meijw@sustech.edu.cn

## I High-field magnetization measurements

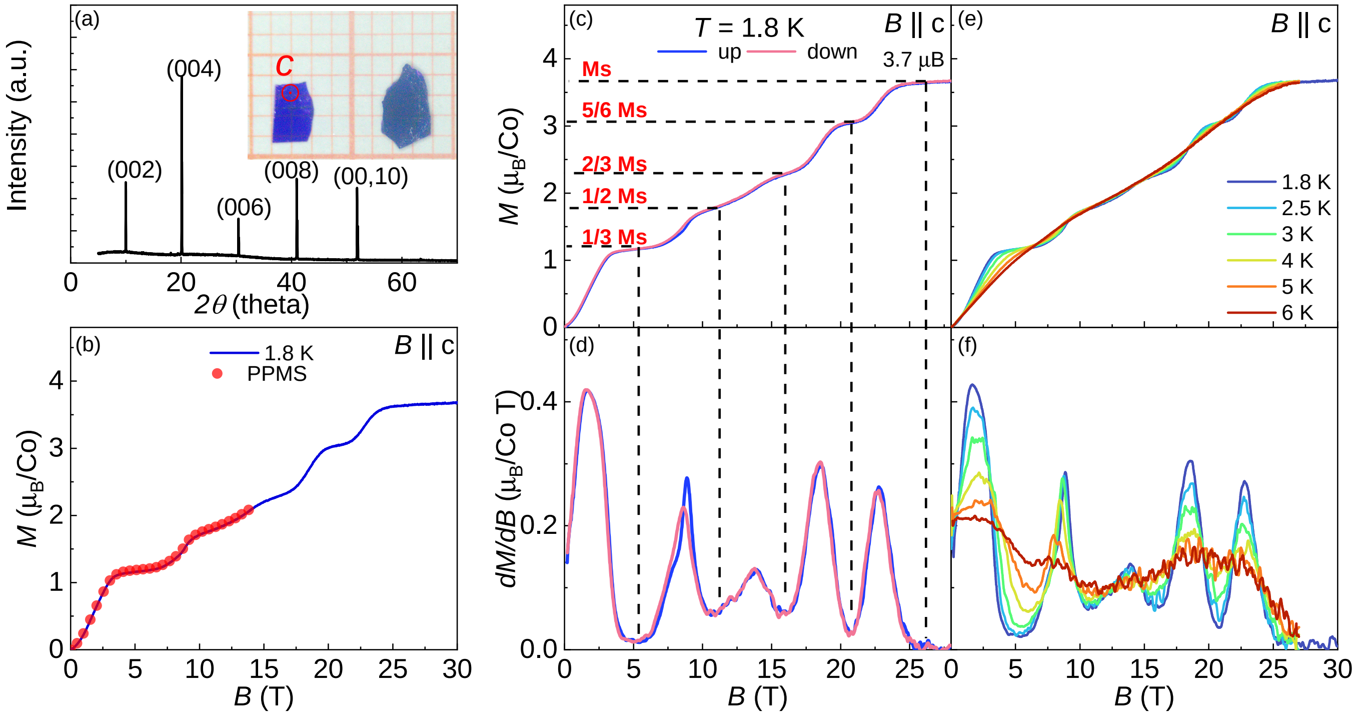


FIG. S1. (a) X-ray diffraction pattern of single crystalline $K_2Co_2(SeO_3)_3$. (b) Comparison of high-field magnetization with PPMS results at 1.8 K, showing excellent agreement. (c) Field-dependent magnetization for increasing and decreasing fields at 1.8 K. (d) Corresponding derivative curves revealing clear hysteresis around 8 T, indicating a first-order phase transition between 1/3 and 1/2 plateaus. (e) Temperature evolution of high-field magnetization curves. (f) Temperature dependence of derivative curves showing the gradual suppression of magnetization plateaus, with the 2/3-plateau being most sensitive to thermal fluctuations.

## II Specific heat analysis

The magnetic contribution to the specific heat was isolated by carefully subtracting the phonon background. The phonon specific heat was modeled using a combined Debye-Einstein model:

$$C_{\text{ph}}(T) = \alpha 9nR\left(\frac{T}{\theta_D}\right)^3 \int_0^{\theta_D/T} \frac{x^4 e^x}{(e^x-1)^2}\,dx + (1-\alpha)3nR\frac{(\theta_E/T)^2 e^{\theta_E/T}}{(e^{\theta_E/T}-1)^2} \tag{S1}$$

$n$ represents the number of atoms per chemical formula unit, while $R$ denotes the universal gas constant with a value of 8.314 J·mol$^{-1}$·K$^{-1}$. $\theta_D$ and $\theta_E$ correspond to the Debye and Einstein temperatures, respectively. The parameter $\alpha$ is utilized to quantify the relative contributions of the Debye and Einstein components to the phonon heat capacity. After fitting specific heat above 30 K, we obtain $\theta_D = 328.94$ K, $\theta_E = 188.87$ K, and $\alpha = 0.716$.

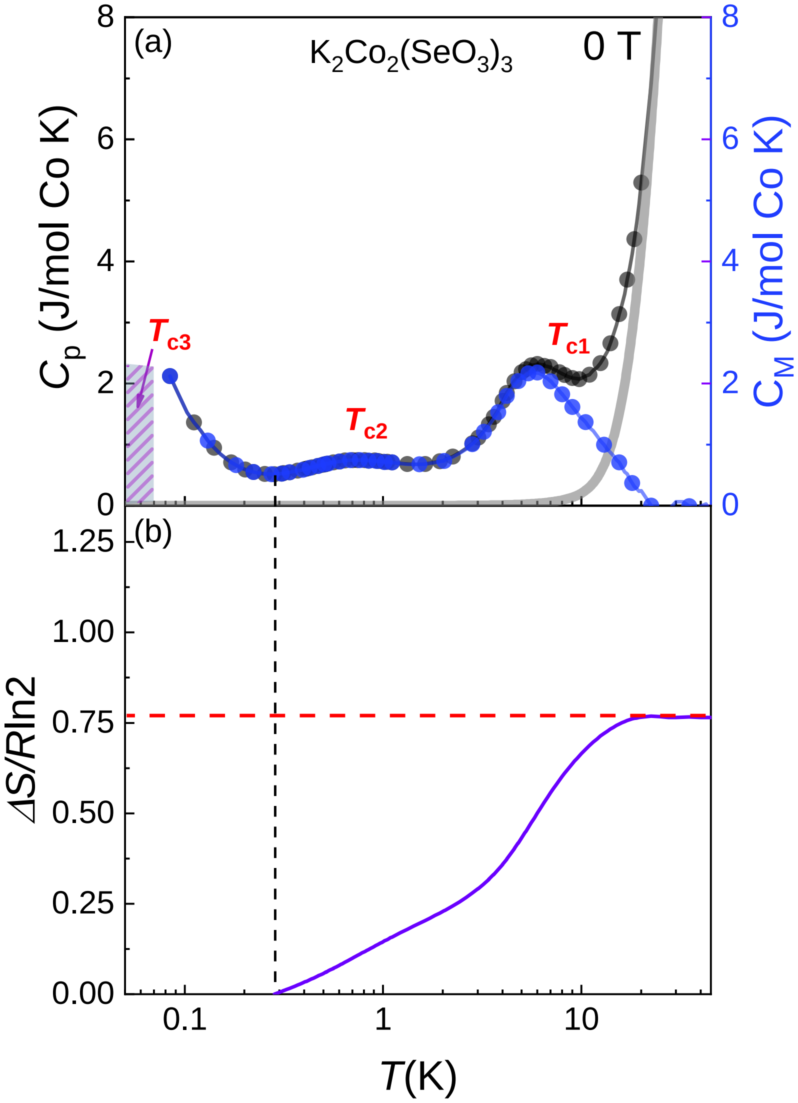


FIG. S2. Zero-field specific heat and entropy. (a) Magnetic specific heat (blue dots) is obtained by subtracting the phonon contribution (gray line) from the total specific heat (black dots). (b) Magnetic entropy integrated over the temperature range from 0.3 K to 30 K, which contains only $0.76R\ln 2$, suggesting an extra entropy of $0.24R\ln 2$ remains for spin dynamics below 0.3 K. Therefore, we conclude that the upturn below 0.3 K is associated with the third phase transition $T_{c3}$.

## III Detailed thermodynamic measurements

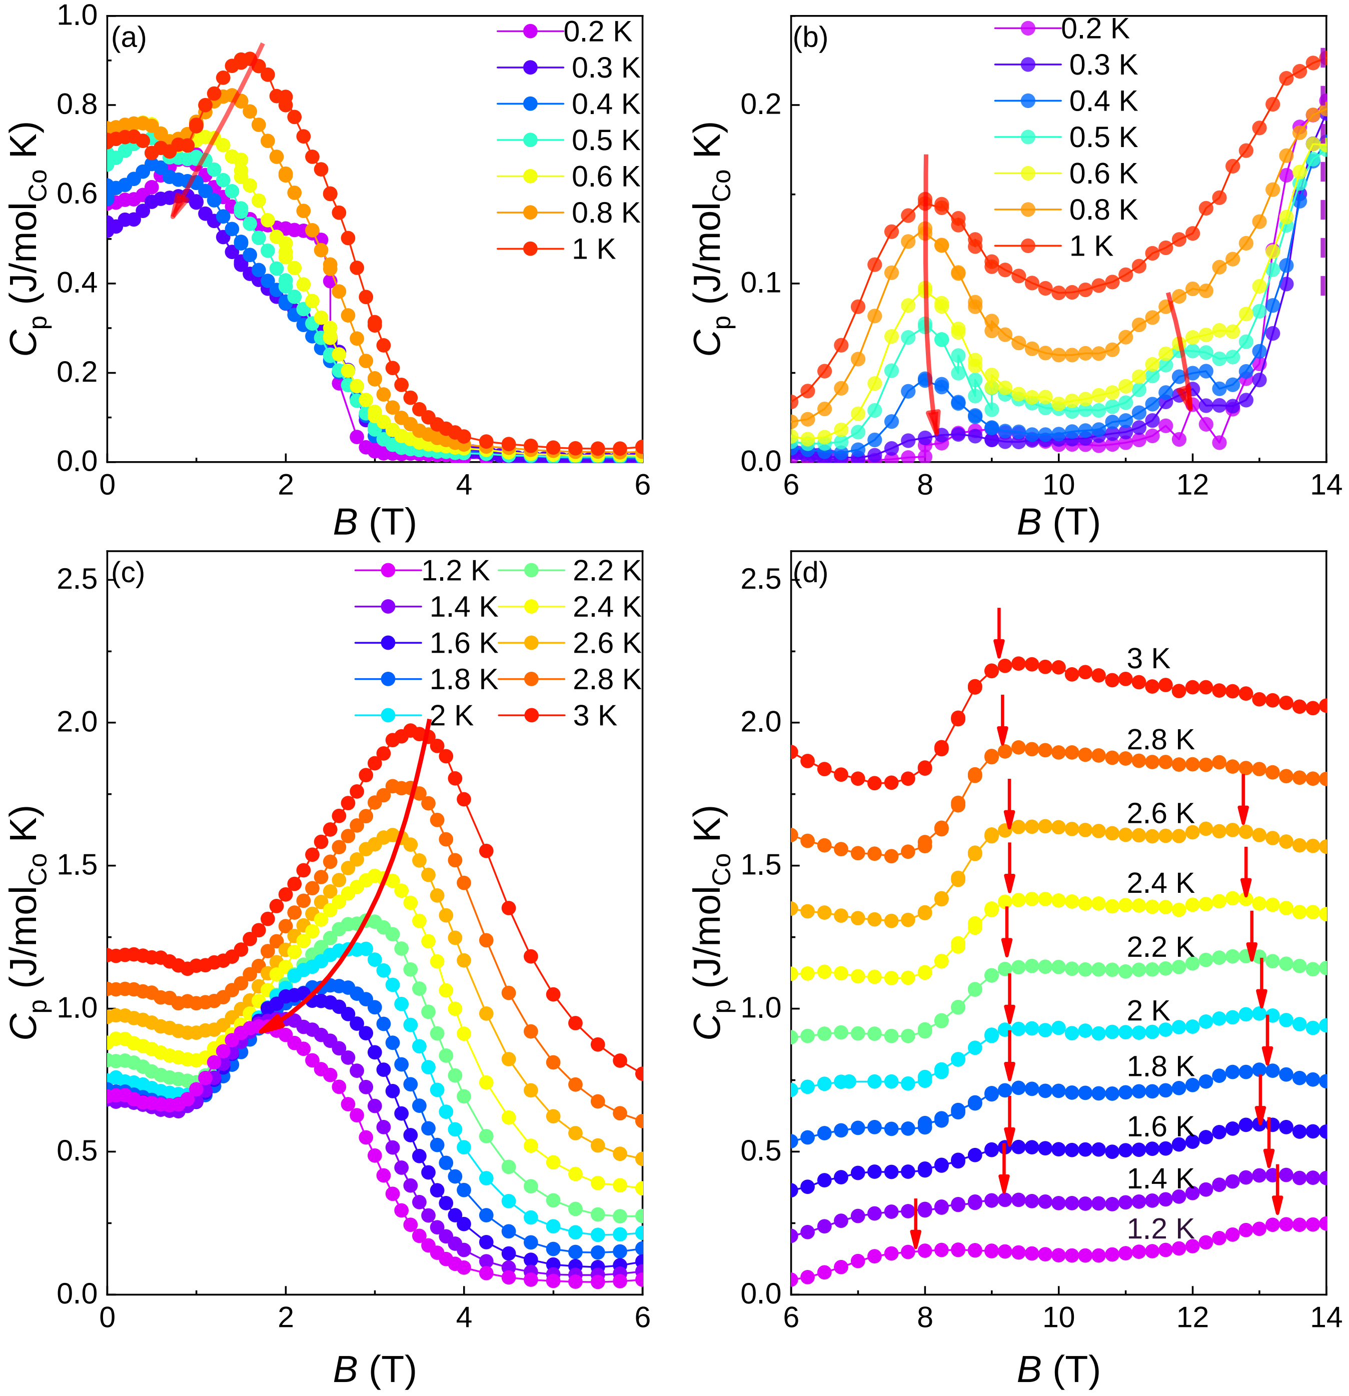


FIG. S3. Field-dependent specific heat measurements of $K_2Co_2(SeO_3)_3$ at various temperatures, extending the data presented in Fig. 3 of the main text. (a) Low-temperature ($T \leq 1$ K) and low-field ($0 < B < 6$ T) regime. (b) Low-temperature ($T \leq 1$ K) and high-field ($6 < B < 14$ T) regime. (c) High-temperature ($T > 1$ K) and low-field ($0 < B < 6$ T) regime. (d) High-temperature ($T > 1$ K) and high-field ($6 < B < 14$ T) regime, with an offset of 0.125 for clarity. Arrows in (a), (b), and (c) indicate the evolution of critical fields, while arrows in (d) denote the critical fields associated with phase transitions.

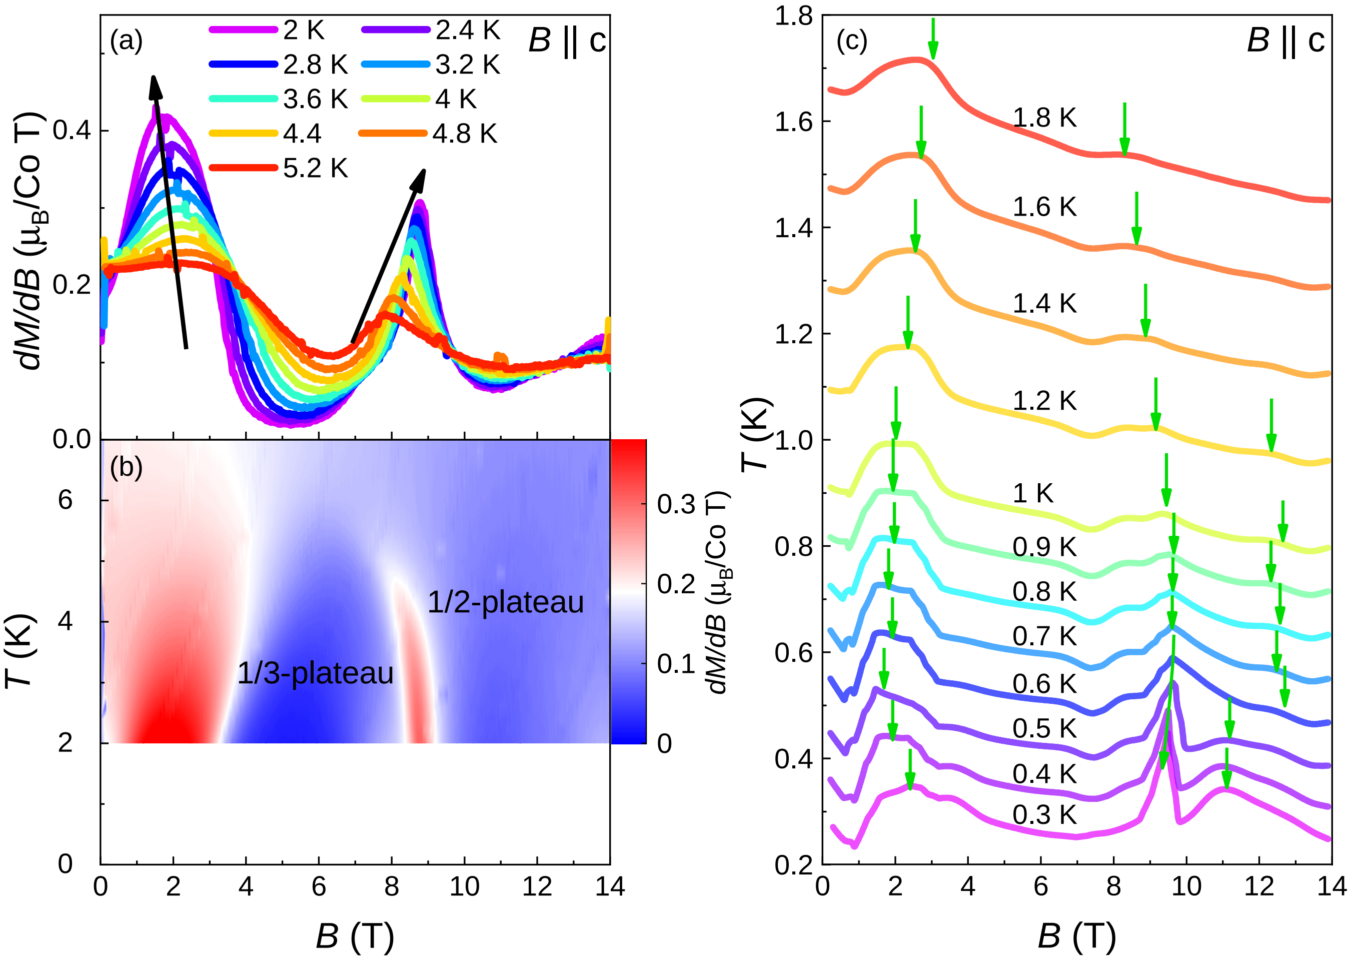


FIG. S4. (a) Derivative curves of field-dependent magnetization ($dM/dB$) for $B \parallel c$ at selected temperatures. The black arrows indicate the critical fields ($B_c$) associated with the $1/3$-plateau and the $1/2$-plateau. (b) Contour plot of $dM/dB$ revealing distinct regions corresponding to the $1/3$-plateau and $1/2$-plateau phases. (c) Magnetocaloric effect (MCE) curves measured under increasing magnetic fields at selected temperatures. Arrows around 2–3 T and 9–10 T correspond to the $1/3$-plateau and $1/2$-plateau phases, respectively. Additional features above 11 T at temperatures below 0.5 K suggest the emergence of a dome-shaped phase associated with the $2/3$-plateau.

## IV Classical Monte Carlo simulations

To capture the multiple magnetization plateaus observed experimentally, we extended our model to include next-nearest-neighbor interactions $J_n$. The complete Hamiltonian is given by:

$$\begin{aligned} H = & \sum_{n\langle ij\rangle} J[(S^x_{ni}S^x_{nj} + S^y_{ni}S^y_{nj})/\Delta + S^z_{ni}S^z_{nj}] \\ & + \sum_i J^0_\perp[(S^x_{1i}S^x_{2i} + S^y_{1i}S^y_{2i})/\Delta + S^z_{1i}S^z_{2i}] \\ & + \sum_{\langle ij\rangle'} J_\perp[(S^x_{1i}S^x_{2j} + S^y_{1i}S^y_{2j})/\Delta + S^z_{1i}S^z_{2j}] \\ & + \sum_{n[ij]} J_n[(S^x_{ni}S^x_{nj} + S^y_{ni}S^y_{nj})/\Delta + S^z_{ni}S^z_{nj}] \\ & - B\sum_i (S^z_{1i} + S^z_{2i}). \end{aligned} \tag{S2}$$

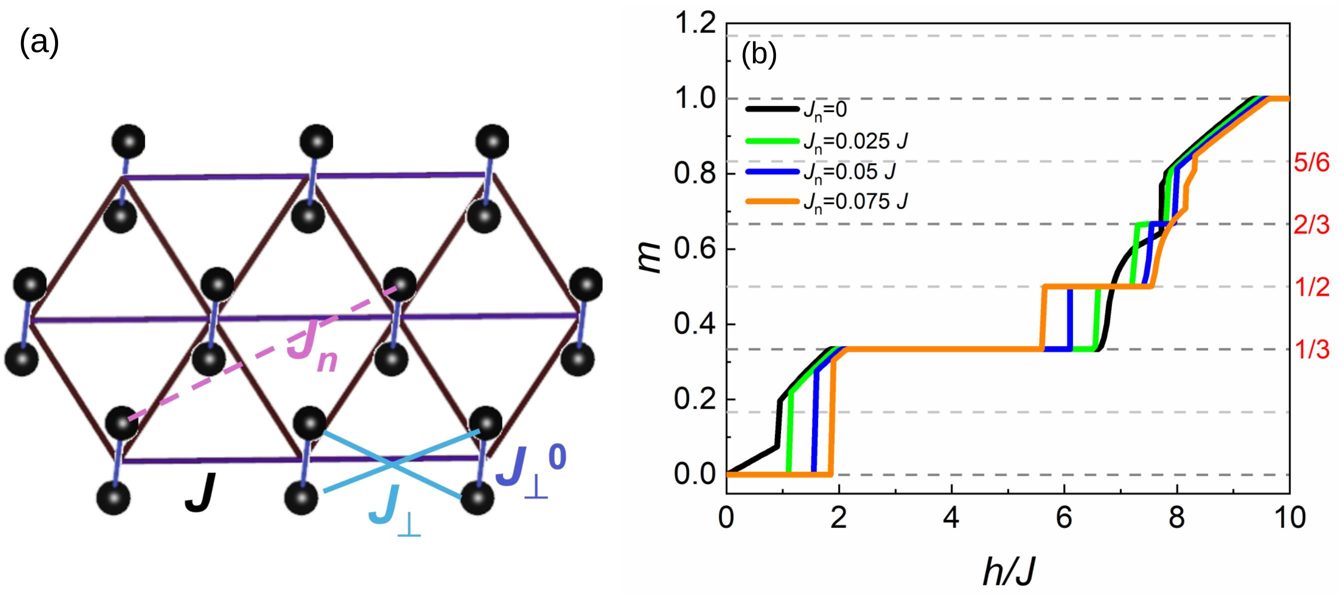


FIG. S5. (a) $J$ and $J_n$ represent the nearest-neighbor and next-nearest-neighbor intralayer interactions, respectively. $J^0_\perp$ denotes the intra-dimer interaction, while $J_\perp$ represents the cross-dimer interaction. (b) Simulations of magnetization plateaus with various $J_n$, and fixed parameters $L = 24$, $J^0_\perp = J$, $J_\perp = 0.2J$, and $\Delta = 3$.
